# Supplementary material for: Short-Range Correlations and the Nuclear EMC Effect in Deuterium and Helium-3
Source: arXiv:2006.10249 ancillary file (2020-07-13)
Supplement: Supplementary file 1 [file supplemental_v0.pdf]

# Supplementary Materials: Short-range correlations and the nuclear EMC effect in Deuterium and Helium-3

## $\chi^2$-MINIMIZATION PROCEDURE

We calculate $F_2^A(x_B)$ for $^3$He and $^2$H in a nuclear convolution approximation:

$$F_2^A(x_B,Q^2) = \int_{x_B}^{A} \frac{d\alpha}{\alpha} \int_{-\infty}^{0} dv\, F_2^p\Big(\tilde{x},Q^2\Big) \left[Z\tilde{\rho}_p^A(\alpha,v) + N\tilde{\rho}_n^A(\alpha,v)\frac{F_2^n}{F_2^p}(\tilde{x})\right] \times \Big(1+v\ f^{off}(\tilde{x})\Big), \tag{1}$$

and form the EMC ratios of $F_2^{^3He}/F_2^d$ to compare to [1] and $F_2^d/(F_2^p+F_2^n)$ to compare to [2] in order to infer parameters of interest. See section **Low $Q^2$, High-$x_B$ Sensitivity** for definition and discussion of $\tilde{x}$. In particular, we would like to investigate the modification function $f^{off}(\tilde{x})$, which we assume to be the same for neutrons and protons, as well as the same across all nuclei. We consider three models:

$$\begin{aligned} f^{off}_{const}(\tilde{x}) &= a_{const}, \\ f^{off}_{lin\ x_B}(\tilde{x}) &= a_{lin\ x_B} + b_{lin\ x_B}\cdot\tilde{x} \\ f^{off}_{KP,\ CJ}(\tilde{x}) &= C(\tilde{x}-x_0)(\tilde{x}-x_1)(1+x_0-\tilde{x}) \end{aligned}$$

To perform parameter inference, we construct the structure function ratios (following Eq. 1) for each kinematic point $i(x_B,Q^2)$ in the data sets considered, i.e. $\frac{F_2^{^3He}}{F_2^d}|_{i,theo}$ and $\frac{F_2^d}{F_2^p+F_2^n}|_{i,theo}$. We allow for a floating re-normalization of the data sets, $N_B$ for [2] and $N_S$ for [1]. We then calculate a $\chi^2$ for the current parameter assumptions $(f^{off}(\tilde{x}), N_B, N_S)$:

$$\begin{aligned} \chi^2 = &\sum_{i\in^2H}\left(\frac{N_B\cdot\frac{F_2^d}{F_2^p+F_2^n}|_{i,theo} - \frac{F_2^d}{F_2^p+F_2^n}|_{i,meas}}{\sigma_i}\right)^2 + \sum_{i\in^3He}\left(\frac{N_S\cdot\frac{F_2^{^3He}}{F_2^d}|_{i,theo} - \frac{F_2^{^3He}}{F_2^d}|_{i,meas}}{\sigma_i}\right)^2 \\ &+\left(\frac{N_B-1}{\sigma_{norm,B}}\right)^2 + \left(\frac{N_S-1}{\sigma_{norm,S}}\right)^2 \end{aligned} \tag{2}$$

and minimize $\chi^2$ to infer our parameters. $F_2^p(\tilde{x},Q^2)$ carries the only $Q^2$ dependence we assume in Eq. 1. We calculated $F_2^p$ using a the GD11-P parameterization [3]. $\tilde{\rho}^A_{p,n}(\alpha,v)$ are the lightcone distributions for protons and neutrons in a given nucleus $A$. The minimization procedure was performed two times: using a spectral function approximation to $\tilde{\rho}(\alpha,v)$ and using the lightcone formalism (see main paper for details).

$F_2^n/F_2^p$ is parameterized as $F_2^n/F_2^p(\tilde{x}) = a_{np}\,(1-\tilde{x})^{b_{np}} + c_{np}$, where there is no explicit $Q^2$ considered. We fit this parameterization to two recent predictions by Segarra [4] and Arrington [5], and then perform the $\chi^2$ minimization using each $F_2^n/F_2^p$ prediction. We do not allow parameter variation of $F_2^n/F_2^p$ in the minimization procedure with the two data sets considered. However, by taking two extreme predictions of $F_2^n/F_2^p$, we can study the sensitivity our results have to the exact nature of $F_2^n/F_2^p$.

In the case of using $f^{off}_{KP,\ CJ}(\tilde{x})$, we fixed the parameters of the offshell function to those found in a minimization by [6] ($f^{off}_{KP}$) and by [7] ($f^{off}_{CJ}$). We note that while the same offshell parameterization is used by both groups, [6] considered a wide range of nuclear DIS data sets and [7] used DIS data on the proton and deuterium to infer their offshell function.

16 minimization trials were performed for the various model assumptions:

a) SF with $F_2^n/F_2^p|_{Seg.}$ with $f^{off}_{const}$

b) SF with $F_2^n/F_2^p|_{Arr.}$ with $f^{off}_{const}$

c) SF with $F_2^n/F_2^p|_{Seg.}$ with $f^{off}_{lin\ x_B}$

d) SF with $F_2^n/F_2^p|_{Arr.}$ with $f^{off}_{lin\ x_B}$

e) SF with $F_2^n/F_2^p|_{Seg.}$ with $f^{off}_{KP}$

f) SF with $F_2^n/F_2^p|_{Arr.}$ with $f^{off}_{KP}$

g) SF with $F_2^n/F_2^p|_{Seg.}$ with $f^{off}_{CJ}$

h) SF with $F_2^n/F_2^p|_{Arr.}$ with $f^{off}_{CJ}$

i) GCF-LC with $F_2^n/F_2^p|_{Seg.}$ with $f^{off}_{const}$

j) GCF-LC with $F_2^n/F_2^p|_{Arr.}$ with $f^{off}_{const}$

k) GCF-LC with $F_2^n/F_2^p|_{Seg.}$ with $f^{off}_{lin\ x_B}$

l) GCF-LC with $F_2^n/F_2^p|_{Arr.}$ with $f^{off}_{lin\ x_B}$

m) GCF-LC with $F_2^n/F_2^p|_{Seg.}$ with $f^{off}_{KP}$

n) GCF-LC with $F_2^n/F_2^p|_{Arr.}$ with $f^{off}_{KP}$

o) GCF-LC with $F_2^n/F_2^p|_{Seg.}$ with $f^{off}_{CJ}$

p) GCF-LC with $F_2^n/F_2^p|_{Arr.}$ with $f^{off}_{CJ}$

where SF is a minimization trial that approximates $\tilde{\rho}(\alpha, v)$ with a spectral-function, GCF-LC is a minimization trial that uses the lightcone formalism for $\tilde{\rho}(\alpha, v)$, $F_2^n/F_2^p|_{Seg.}$ is a minimization trial that uses $F_2^n/F_2^p$ fitted to [4], and $F_2^n/F_2^p|_{Arr.}$ uses a fit to [5].

## SF AND GCF-LC COMPARISON

The distributions $\tilde{\rho}(\alpha, v)/\alpha$ of lightcone fraction and virtuality as shown below for deuteron in Fig. 1 and helium-3 in Fig. 2, using both the GCF lightcone formalism (GCF-LC) and the spectral function formalism (SF). We note that the largest deviations between these models occurs at large virtuality, in the SRC-dominated region. The SF model has increased probability of low-$\alpha$ nucleons relative to the GCF-LC model. In both formalisms, a momentum cutoff was placed at $p = 1$ GeV/$c$ due to the expectation that assumptions would break down beyond this region. The hard cuts seen at large $-v$ are the result of this cutoff, which is expressed differently in the GCF-LC model and the SF model.

Fig. 3 shows the distribution $\tilde{\rho}(\alpha)/\alpha$ of the lightcone fraction for all nucleons (integrated over $v$), for deuteron and both protons and neutrons in helium-3. While the GCF-LC formalism produces lightcone fraction distributions that are symmetric around $\alpha = 1$, this symmetry is not manifest in the SF formalism, resulting in the small momentum sum-rule violation mentioned in the main text.

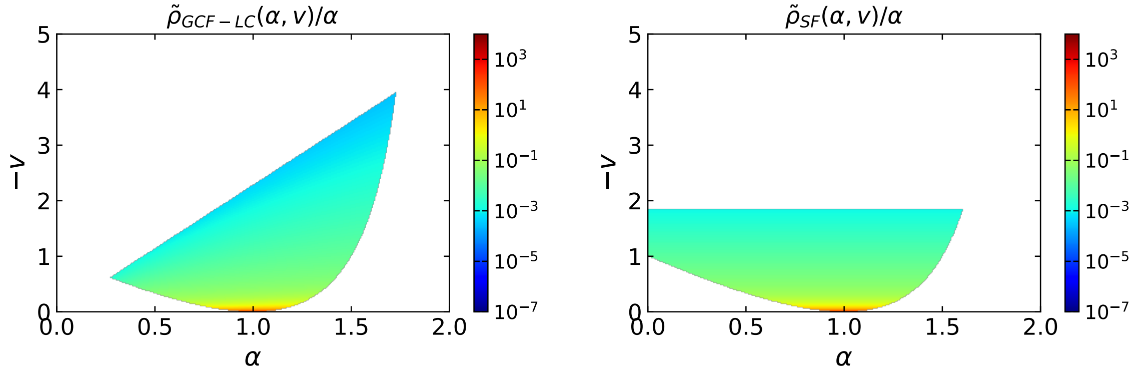


FIG. 1: Comparison of $\tilde{\rho}^{^2H}_{p,n}(\alpha, v)$ for the GCF-LC formalism and SF formalism. Due to isospin symmetry, the distributions are identical for proton and neutron

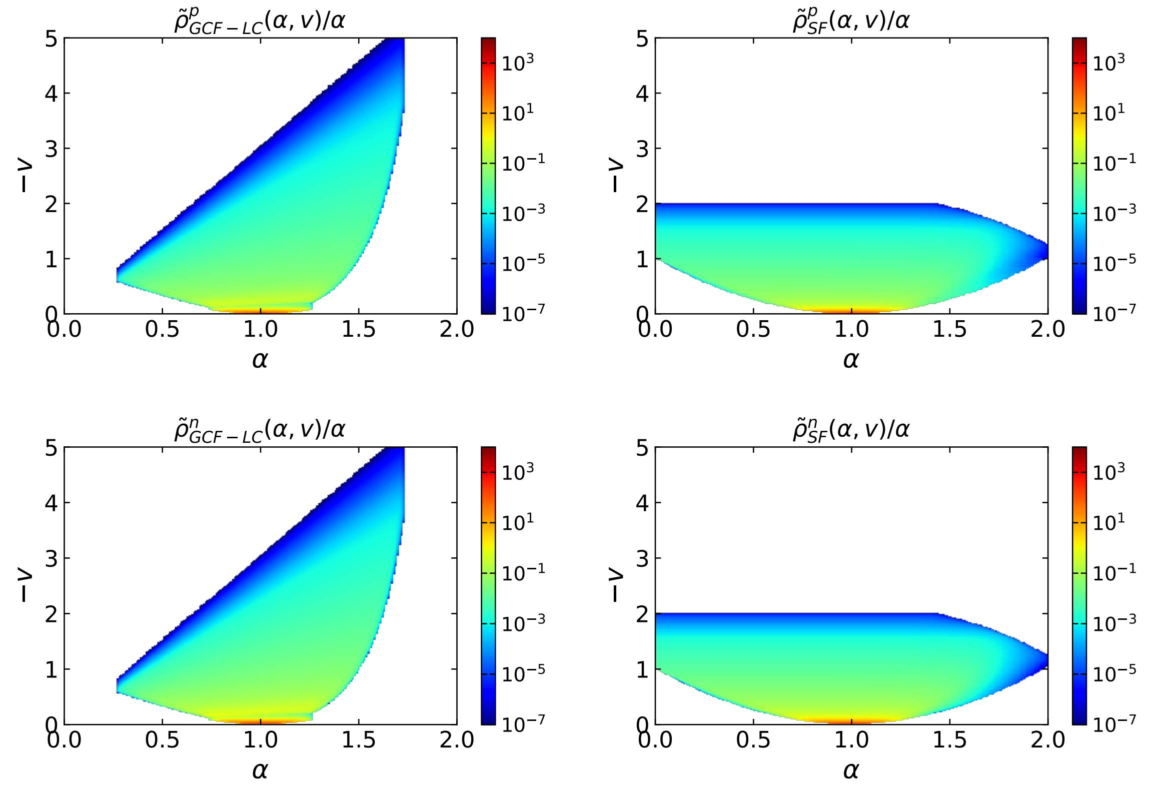


FIG. 2: Comparison of $\tilde{\rho}^{^3He}_{p,n}(\alpha, v)$ for the GCF-LC formalism and SF formalism. Proton distributions are shown above and neutron distributions are shown below.

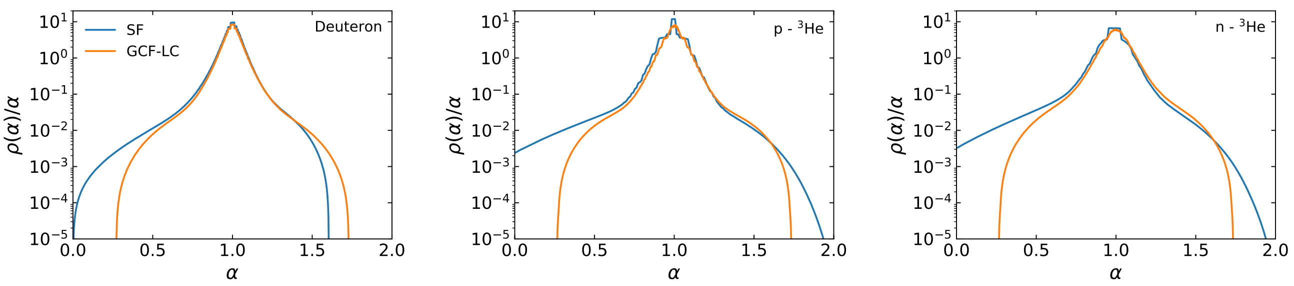


FIG. 3: Lightcone fraction distribution $\tilde{\rho}(\alpha)$ for deuteron (left), protons in helium-3 (center), and neutrons in helium-3 (right).

## QUALITY OF MODEL EXTRACTION

Each minimization trial is shown individually with the data used here with the resulting reduced $\chi^2$:

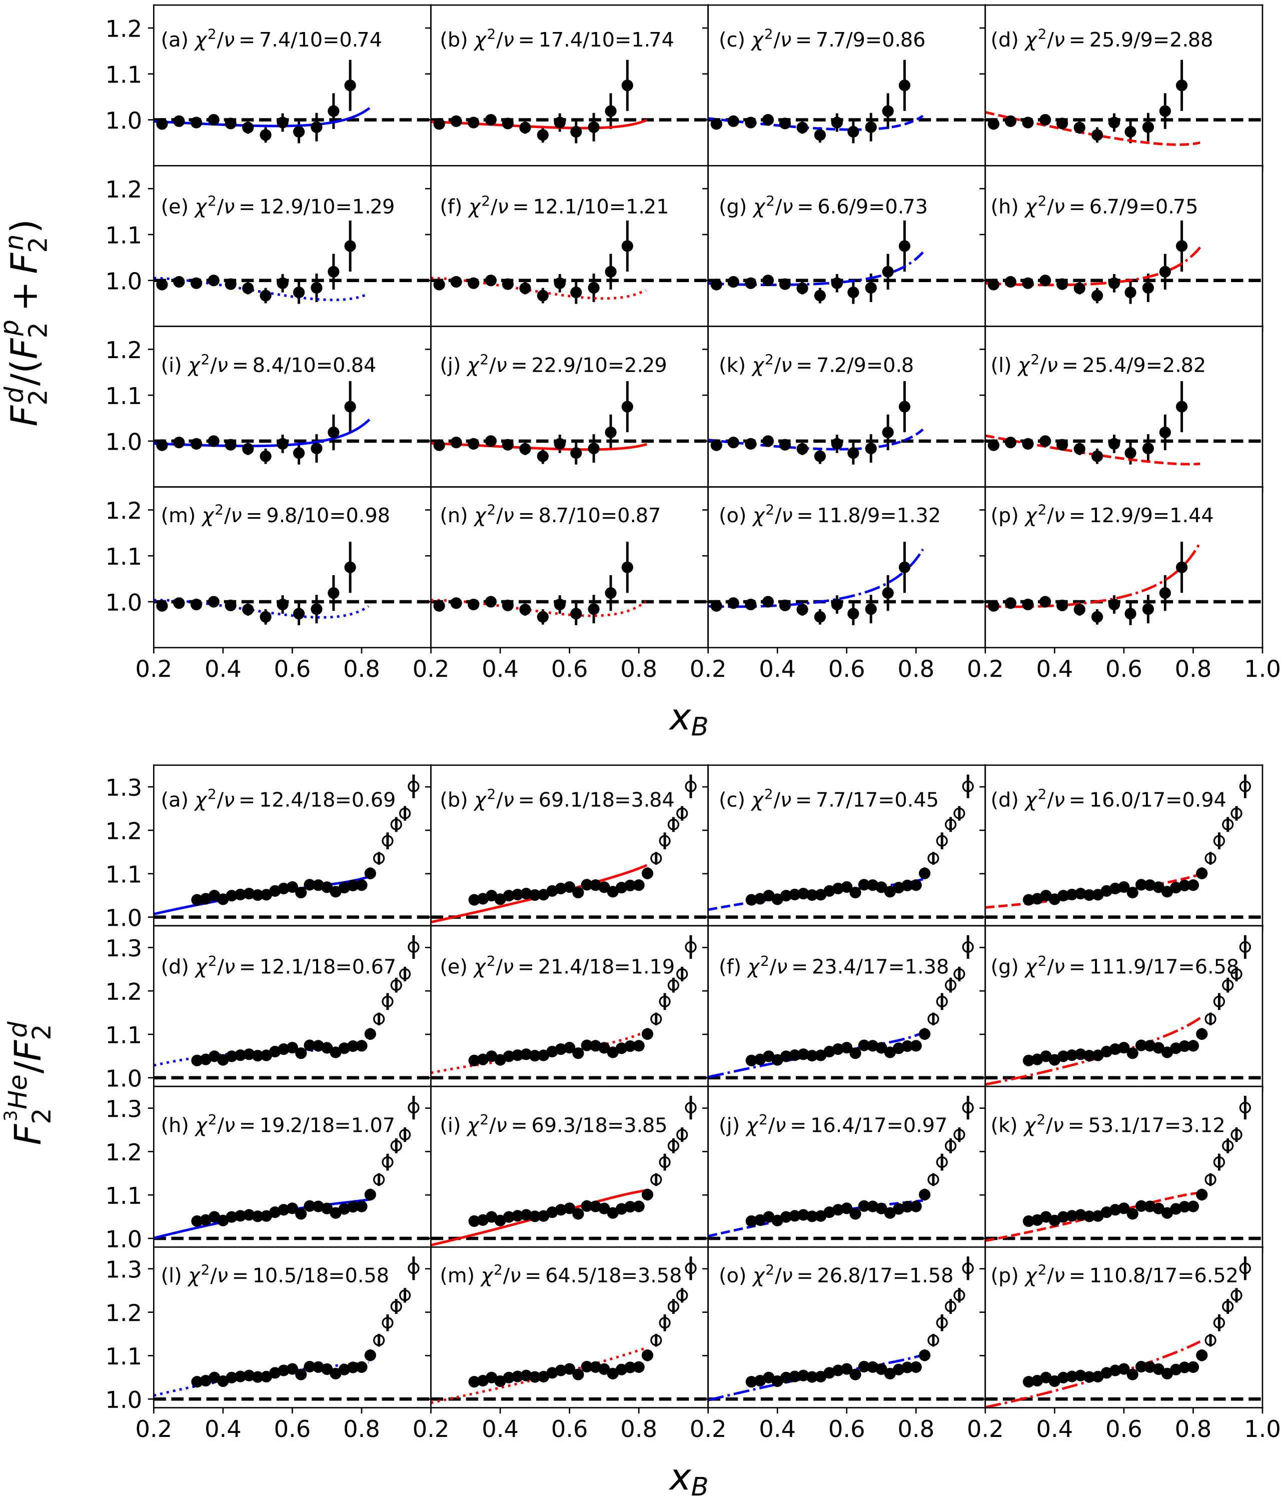


FIG. 4: Fit results using model assumptions described in $\chi^2$**-Minimization Procedure**. Top: fit quality to $F_2^d/(F_2^p + F_2^n)$ data. Bottom: fit quality to $F_2^{^3He}/F_2^d$ data.

## LOW $Q^2$, HIGH-$x_B$ SENSITIVITY

In Eq. 1 of the main text, $\tilde{x}$ is used in the convolution. This arises from an inclusion of the motion of the nucleon within the nucleus, but at low $Q^2$, high-$x_B$, additional terms are needed other than those stated in the main text. Defining $q = (\nu, 0, 0, -|\mathbf{q}|)$, we then express the momenta of the virtual photon and the struck nucleon in the frame:

$$\begin{aligned} q =& \Big(q_- = (q_0 - q_3)\ ,\ q_+ = (q_0 + q_3)\ ,\ \mathbf{q_t} = \mathbf{0}\Big) \\ p =& \Big(p_- = (p_0 - p_3)/m_N\ ,\ p_+ = (p_0 + p_3)/m_N\ ,\ \mathbf{p_t}\Big), \end{aligned} \tag{3}$$

where in this frame, $q_0 = \nu, q_3 = |\mathbf{q}|$. Defining $\tilde{x}$:

$$\begin{aligned} \tilde{x} &= \frac{Q^2}{2(q\cdot p)} = \frac{Q^2}{2\left(\left[q_+\cdot p_-\right]/2 + \left[q_-\cdot p_+\right]/2 - \mathbf{q_t}\cdot\mathbf{p_t}\right)} \\ &= \frac{Q^2}{\left[q_+\cdot p_-\right] + \left[q_-\cdot p_+\right]}. \end{aligned} \tag{4}$$

In the Bjorken frame, $\frac{q_+}{q_-} \to 0$ such that $\tilde{x} \to Q^2/(q_-\cdot p_+)$. With fixed $x_B = Q^2/(2m_N\nu)$, $x_B \to Q^2/m_N q_-$:

$$\begin{aligned} \tilde{x} &= \frac{Q^2}{q_-\cdot p_+} = \frac{x_B}{p_+}m_N \\ &= \frac{x_B}{\alpha}\frac{Am_N}{m_A}, \end{aligned} \tag{5}$$

where $\alpha = Ap_+/m_A$, and we've arrived at the expression used in Eq. 1 in the main text. As the data considered in our fit is at low-$Q^2$, we can directly use Eq. 4. We repeated our minimization procedures and no significant difference was seen in the ratios $F_2^d/(F_2^p + F_2^n)$ , $F_2^{^3He}/F_2^d$ – see Fig. 5

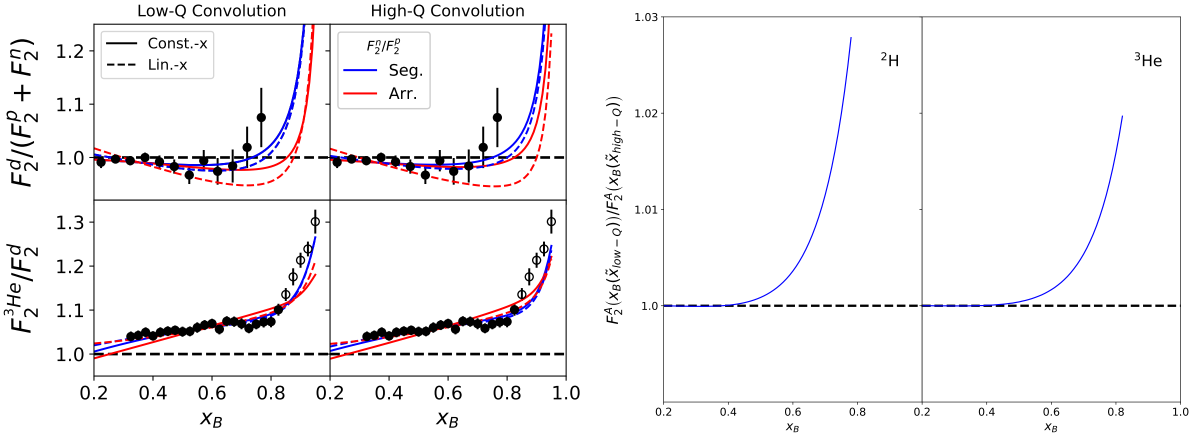


FIG. 5: (left) Convolution results using the finite-energy expression of Eq. 4 for $\tilde{x}$ (Low-Q Convolution) and Bjorken frame of Eq. 5 for $\tilde{x}$ (High-Q Convolution) for deuterium and helium-3. (right) The ratio of structure functions $F_2^A(x_B)$ calculated with Eq. 4 to that calculated with Eq. 5. While at high-$x_B$, the ratio starts to diverge above 2%, we only consider data up to $x_B \sim 0.8$. Our results are robust to which expression is used for $\tilde{x}$ in the convolution.

## CONVOLUTION DECOMPOSITION

### Ratio decomposition

In calculating Eq. 1, we would like to understand the role of low- and high-momentum nucleons. In particular, we'd like to answer how much do high-momentum nucleons contribute to the structure function ratio, especially at

high-$x_B$. In the GCF-LC formalism, $\tilde{\rho}(\alpha, v)$ is already factorized into mean-field/low-momentum (MF) and short-range-correlation/high-momentum (SRC) contributions. In the SF approximation, we simply choose integral bounds of the spectral function for the momentum range of interest (we chose 200 MeV/c):

$$\tilde{\rho}_{N,SF}^{SRC,A}(\alpha, v) = \int_{|\mathbf{p}|=200\text{MeV/c}}^{1000\text{MeV/c}} dEd^3\mathbf{p} \;\; S_N^A(E,p) \cdot \frac{E+p_z}{E} \cdot \frac{m_A}{m_N A} \, \delta\left(\frac{m_N \alpha}{m_A} - \frac{p^+}{P^+}\right) \delta\left(v - \frac{E^2 - |\mathbf{p}|^2 - m_N^2}{m_N^2}\right),$$

and similarly, a $\tilde{\rho}_{N,SF}^{MF,A}(\alpha, v)$ is defined by integrating from $0-200$ MeV/c. Substituting in $\tilde{\rho}_N^{SRC,A}(\alpha, v)$ into Eq. 1, we can calculate $F_2^{SRC,A}$, the contribution to $F_2^A$ by SRC nucleons. We note that $F_2^{MF,A} + F_2^{SRC,A} = F_2^A$. Fig. 7 shows the individual contributions to $F_2^A$ by MF and SRC nucleons (in the main text, the ratio of SRC/MF was taken).

### Offshell decomposition

We would also like to understand the role of high momentum nucleons in the offshell effect $f^{off}(\tilde{x})$ and how that contributes to the overall structure function. We can estimate the offshell contribution to the structure function by taking $F_2^A$(offshell) = $F_2^A$(full) − $F_2^A$no-offshell), where we calculate $F_2^A$(full) by usual means of Eq. 1 and $F_2^A$(no-offshell) is calculated by setting $f^{off}(\tilde{x}) = 0$ in Eq. 1. We then can look again at the contributions due to MF and SRC nucleons to $F_2^A$(offshell). Fig. 8 shows the individual contributions to $F_2^A$(offshell) by MF and SRC nucleons (in the main text, only a select few curves were shown).

## UNIVERSAL FUNCTION PREDICTION

We note that the UMF extracted by Ref. [4, 8] is reproduced with the convolution framework used here for $^3$He, see Fig. 6.

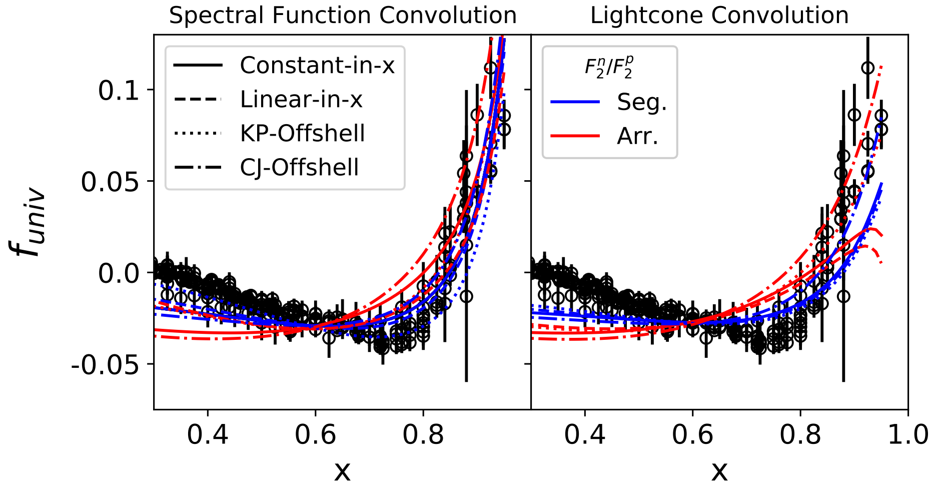


FIG. 6: Convolution results for $^3$He shown as the universal modification function as described in [4], which was unable to decompose nucleon offshell and motion effects. All curves are calculated and extrapolated with the same $Q^2$ as the data for $^3$He.

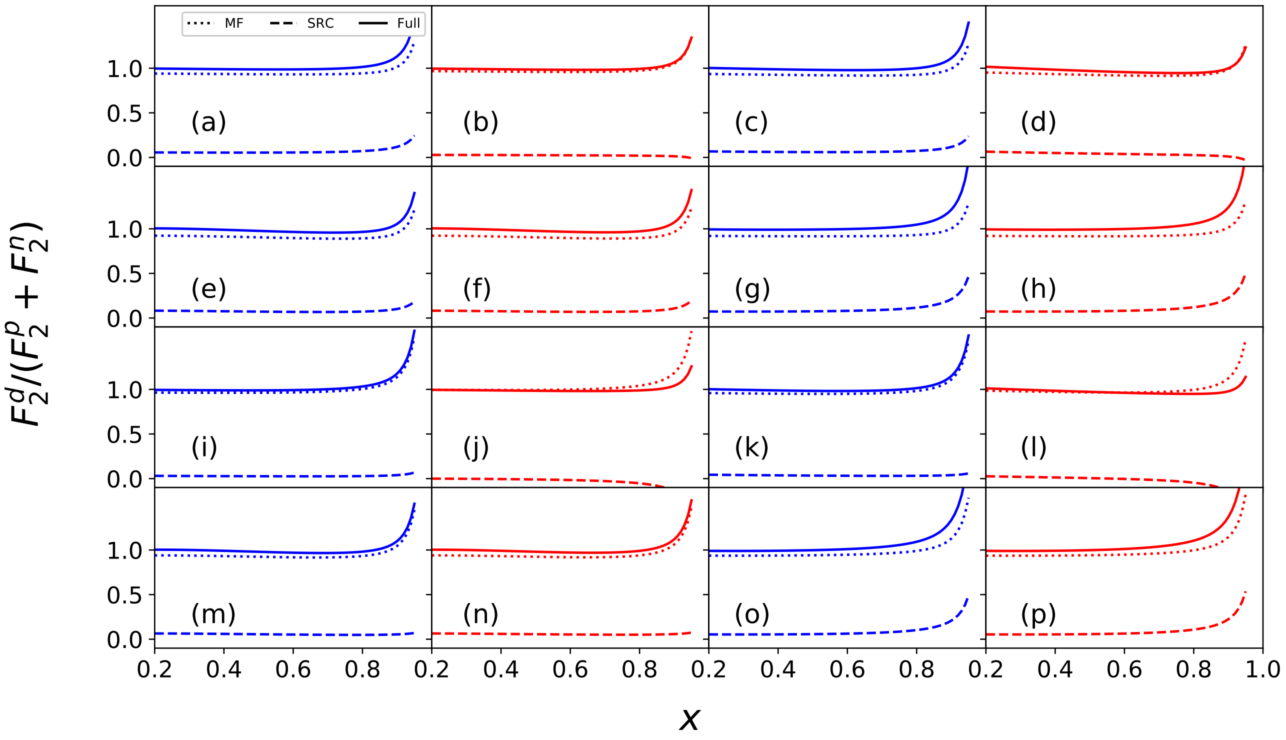


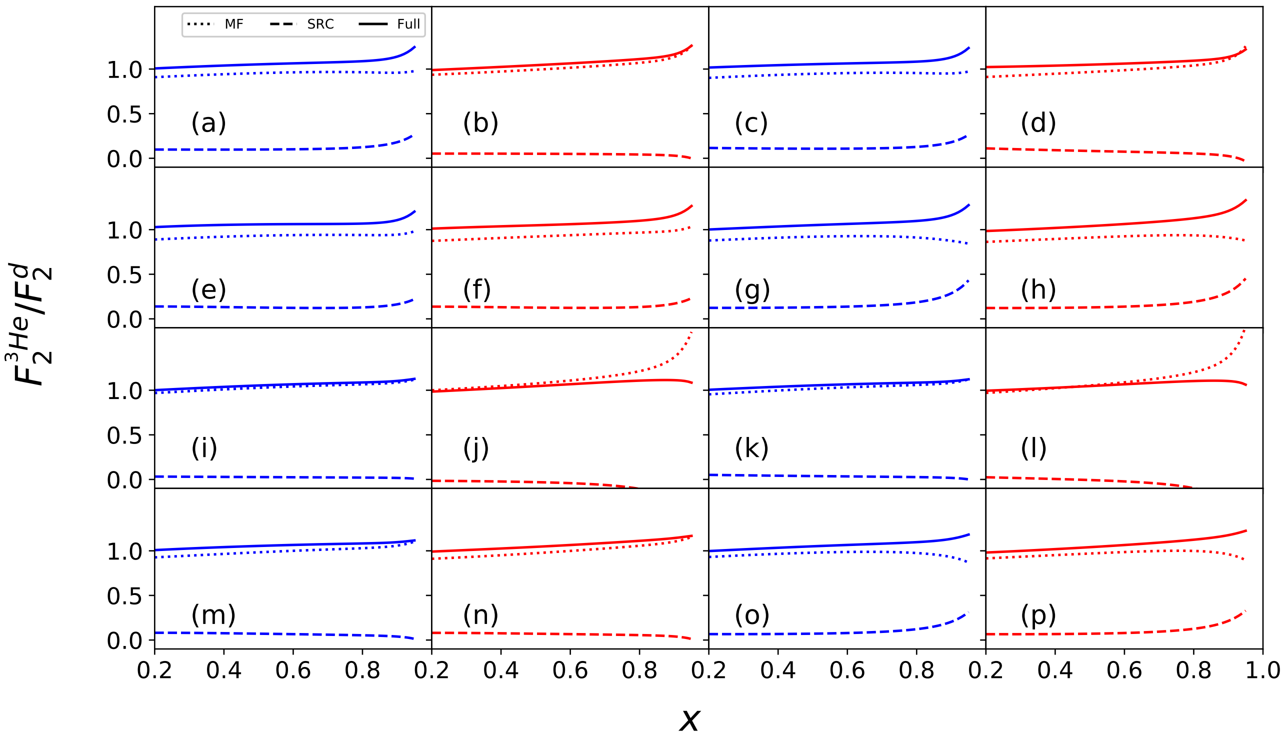


FIG. 7: Decomposition of EMC ratios (Top: deuterium, Bottom: helium-3) for MF (finely dotted lines) and SRC (dashed lines) nucleons, compared to the full (solid lines) convolution. See **Ratio decomposition** for details on calculations. In all curves we see that MF dominates the ratio and the SRC contribution is only $\mathcal{O}(\sim 10\%)$

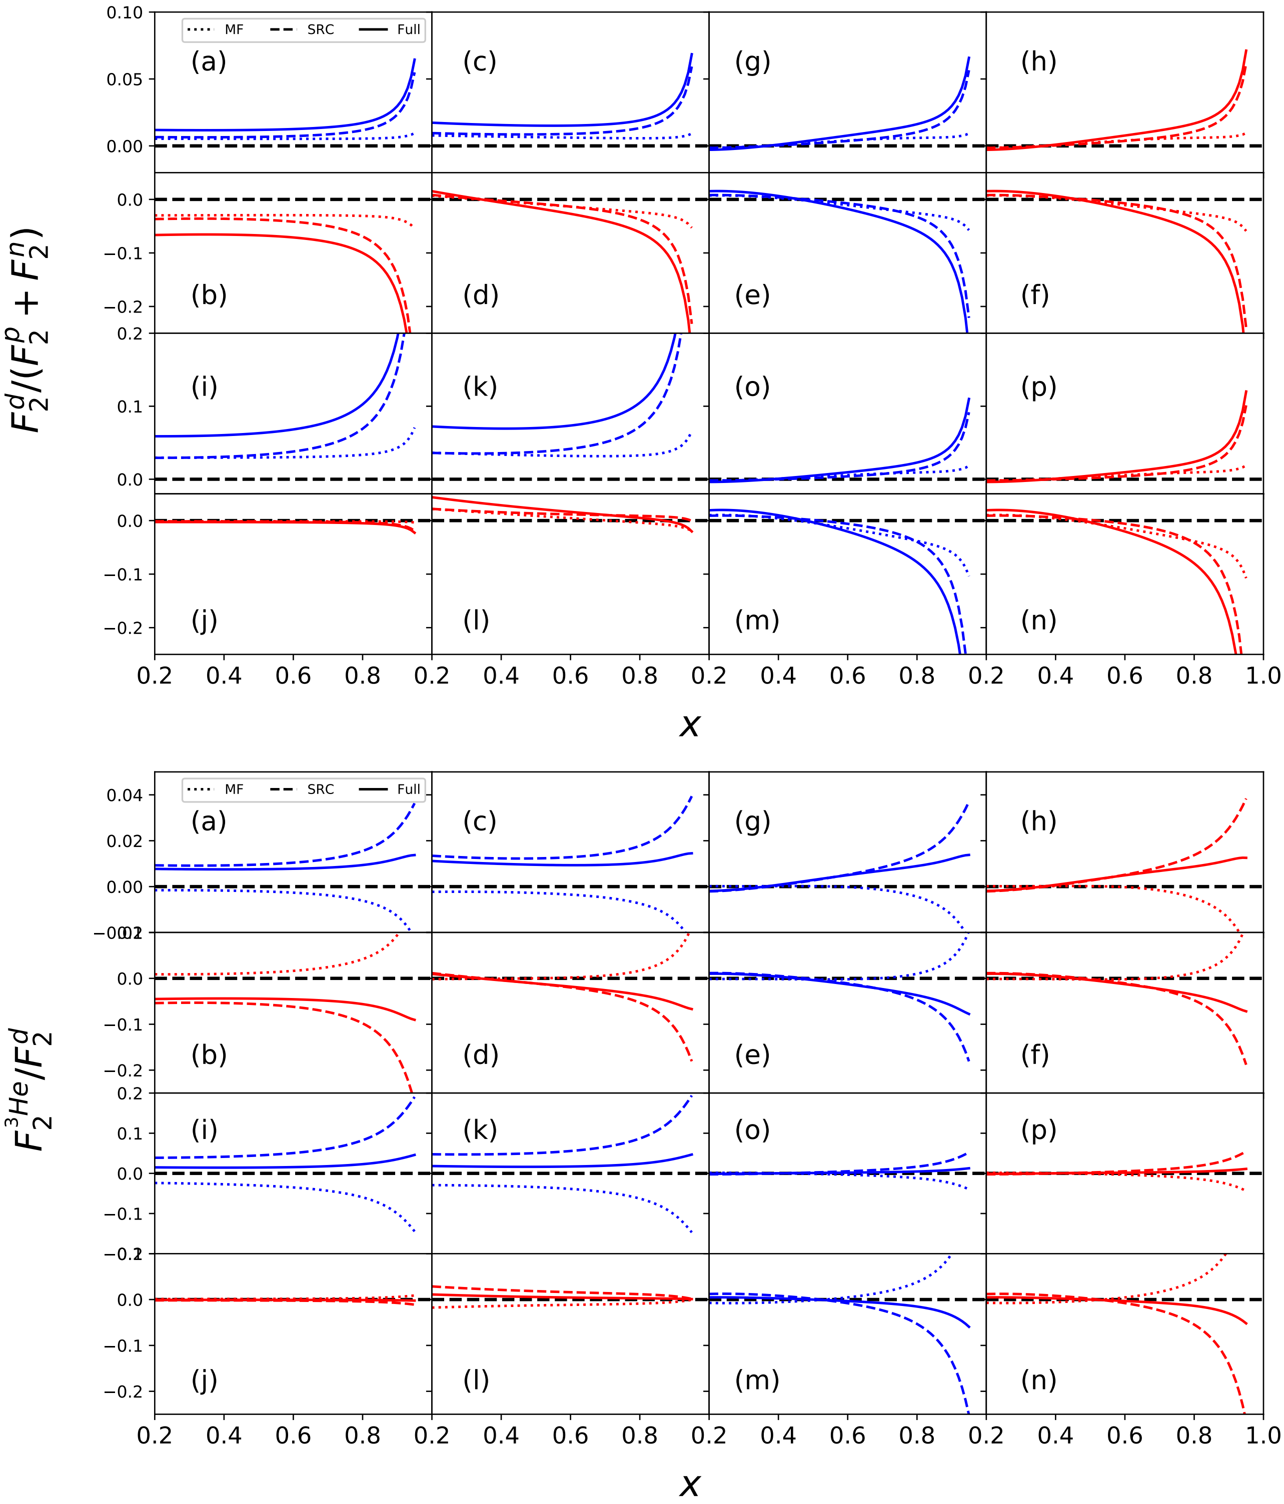


FIG. 8: Decomposition of offshell contribution to ratio (Top: deuterium, Bottom: helium-3) for MF (finely dotted lines) and SRC (dashed lines) nucleons, compared to the full (solid lines) convolution. See **Offshell decomposition** for details on calculations. In all curves we see that now SRC dominates the contribution at high-$x_B$ and the MF contribution is small.

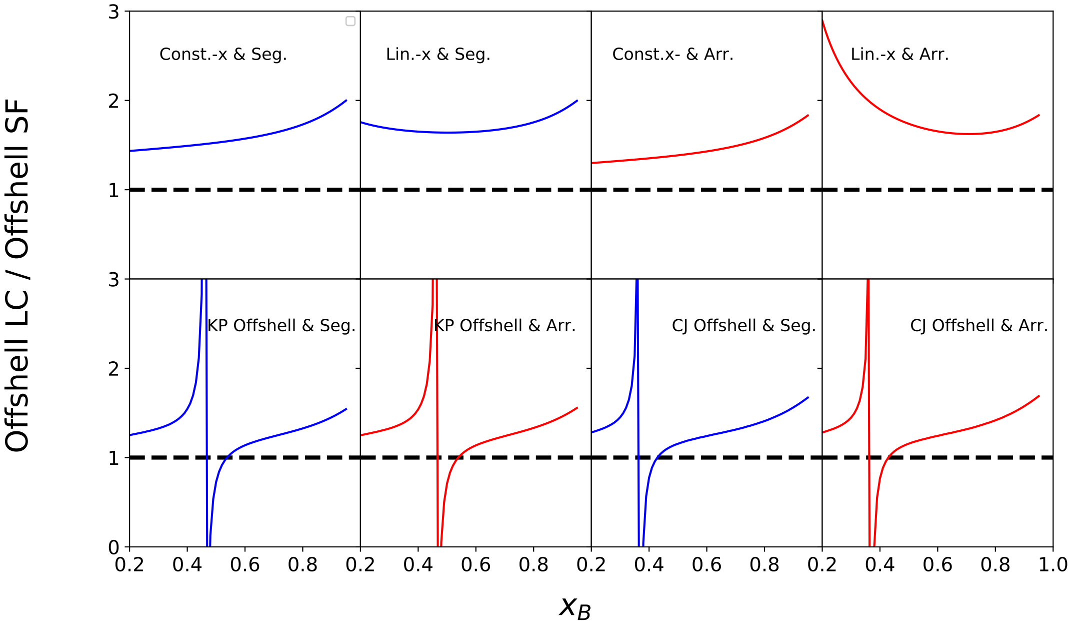


FIG. 9: Ratio of offshell contribution to the structure function in the GCF-LC framework to SF framework. The ratio is always larger than one, signifying that the offshell effect is larger in the GCF-LC framework than SF framework, as expected due to the momentum sum rule violation in the SF framework.

[1] J. Seely *et al.*, Phys. Rev. Lett. **103**, 202301 (2009).
[2] K. A. Griffioen *et al.*, Phys. Rev. **C92**, 015211 (2015), arXiv:1506.00871 [hep-ph] .
[3] A. Airapetian, N. Akopov, and Z. e. a. Akopov, J. High Energ. Phys. **126** (2011), 10.1007/JHEP05(2011)126.
[4] E. P. Segarra, A. Schmidt, D. W. Higinbotham, E. Piasetzky, M. Strikman, L. B. Weinstein, and O. Hen, Phys. Rev. Lett. (2020), arXiv:1908.02223 [nucl-th] .
[5] J. Arrington, J. G. Rubin, and W. Melnitchouk, Phys. Rev. Lett. **108**, 252001 (2012), arXiv:1110.3362 [hep-ph] .
[6] S. Kulagin and R. Petti, Nuclear Physics A **765**, 126 (2006).
[7] A. Accardi, L. T. Brady, W. Melnitchouk, J. F. Owens, and N. Sato, Phys. Rev. **D93**, 114017 (2016), arXiv:1602.03154 [hep-ph] .
[8] B. Schmookler *et al.* (CLAS Collaboration), Nature **566**, 354 (2019).
